# Supplementary material for: Fully automated primary particle size analysis of agglomerates on transmission electron microscopy images via artificial neural networks
Source: arXiv:1806.04010 ancillary file (2018-06-08)
Supplement: Supplementary file 1 [file Supplementary_data.pdf]

# Supplementary data: Fully automated primary particle size analysis of agglomerates on transmission electron microscopy images via artificial neural networks

M. Frei*, F.E. Kruis

*Institute of Technology for Nanostructures (NST) and Center for Nanointegration Duisburg-Essen (CENIDE)*
*University of Duisburg-Essen, Duisburg, D-47057, Germany*

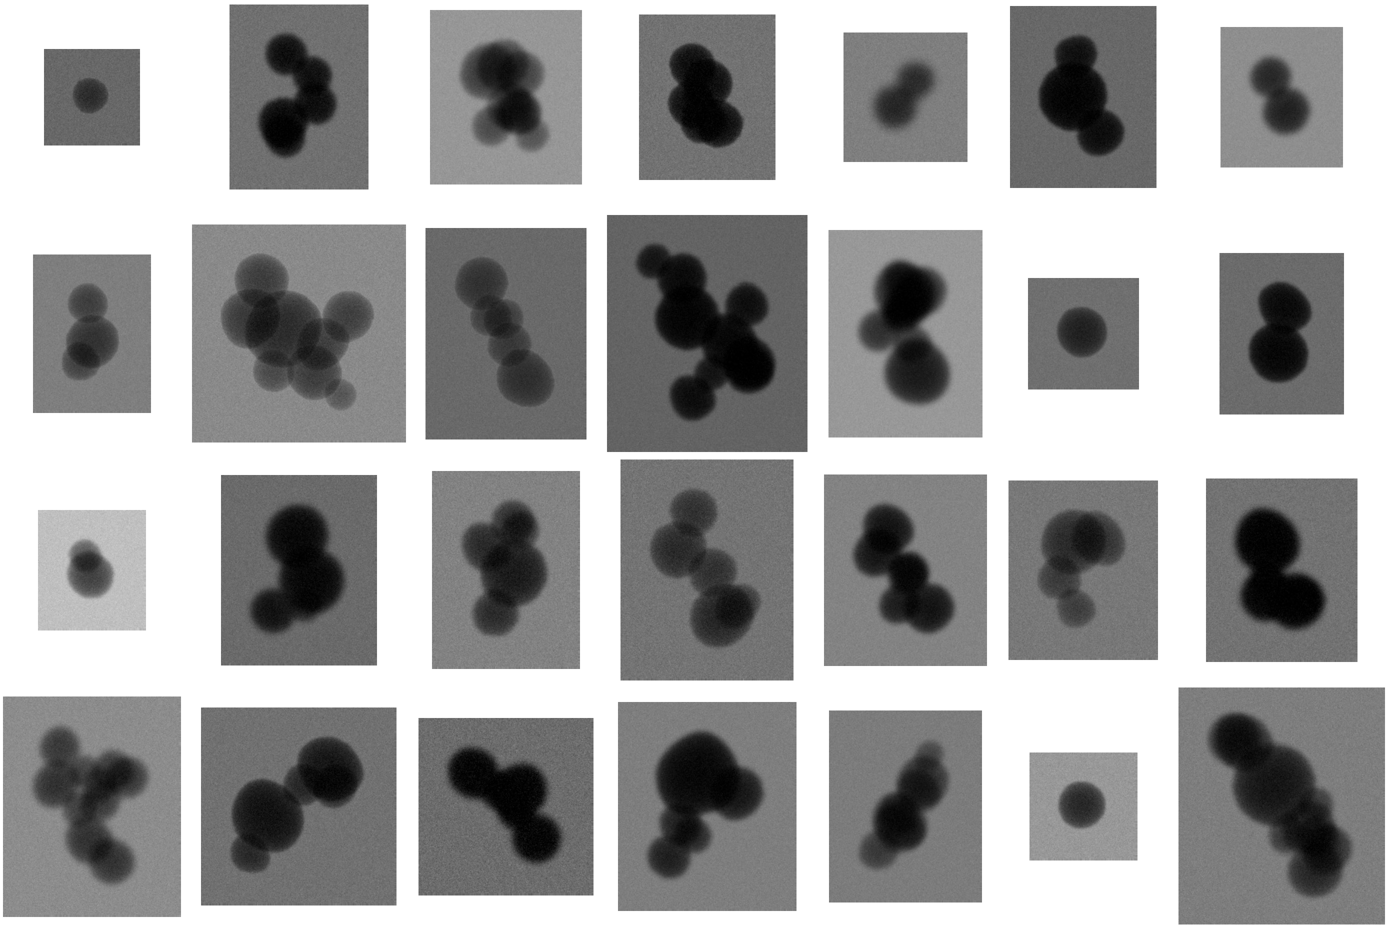

Figure 1: Random selection of synthetic transmission electron microscopy images.

*Corresponding author. Tel.: +49 203 379–3621
*Email address:* max.frei@uni-due.de (M. Frei)

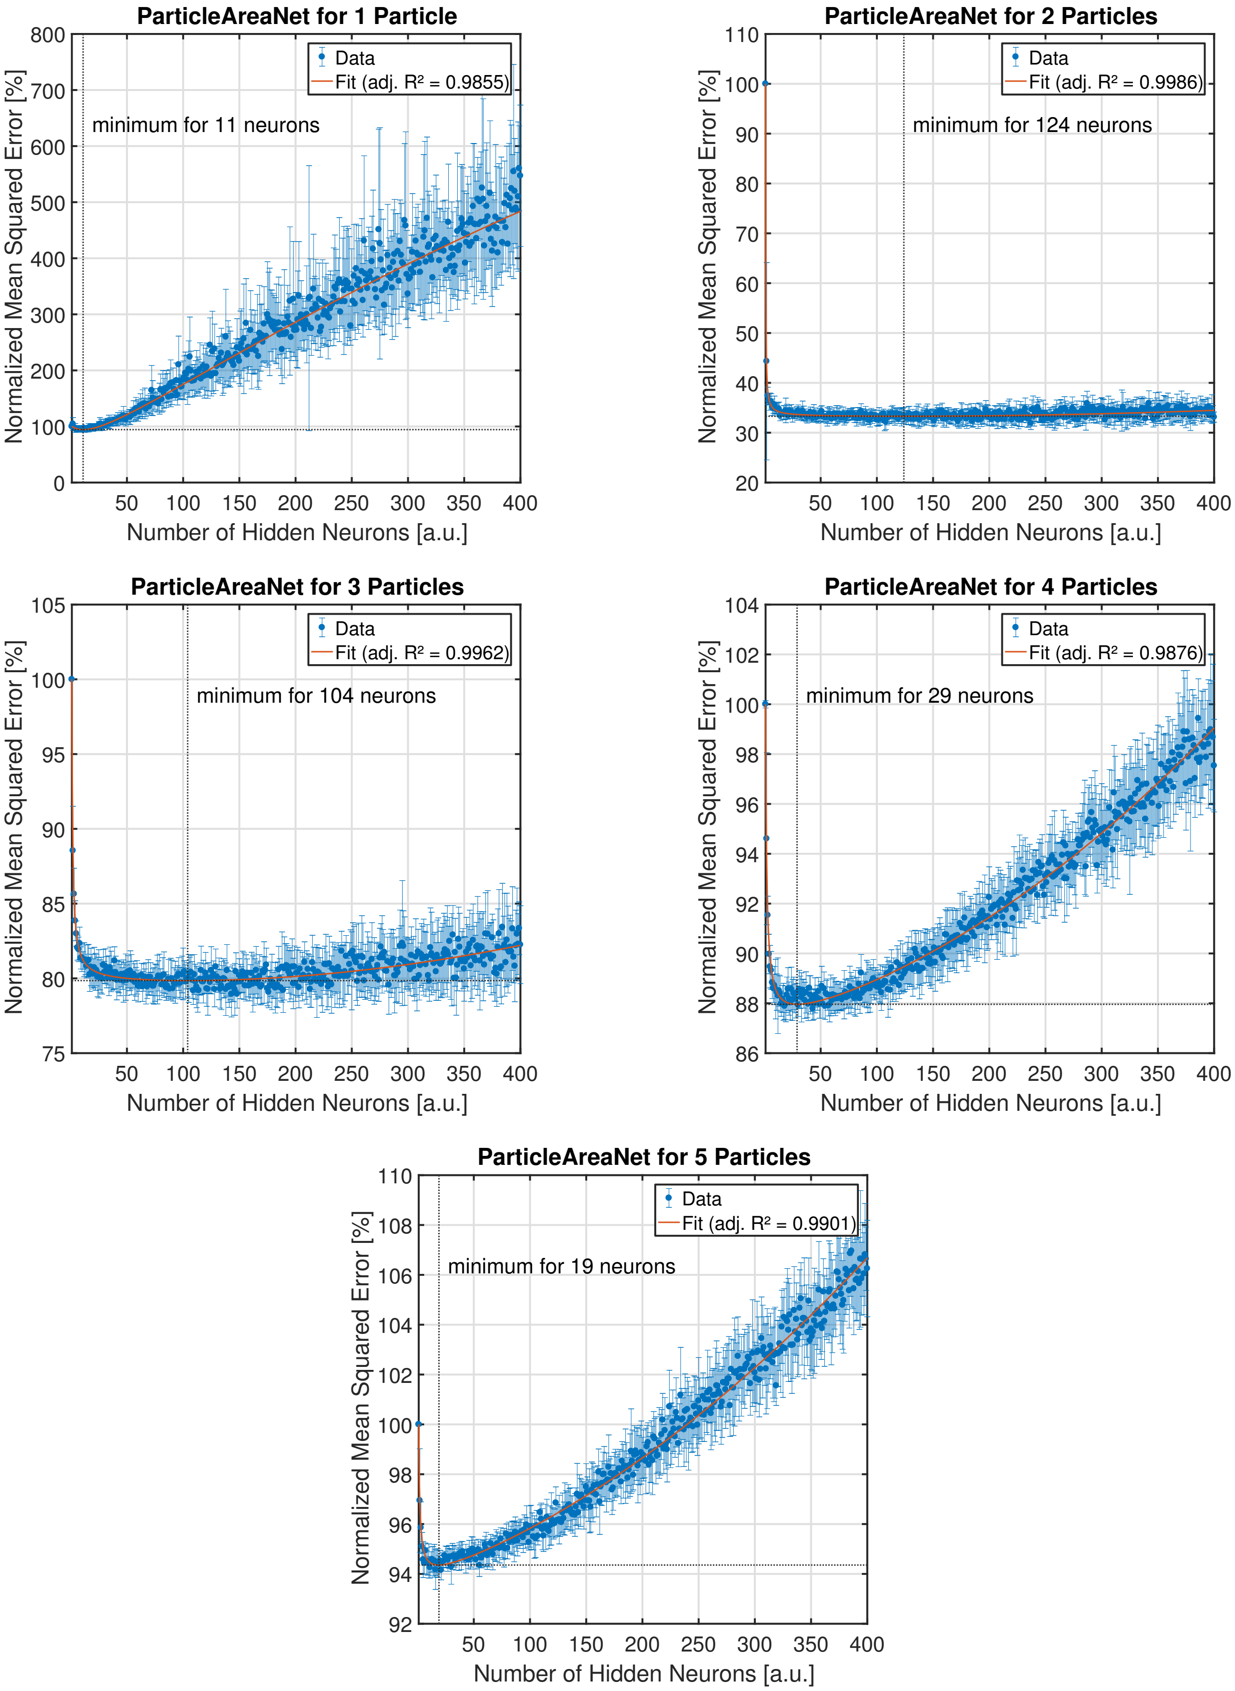


Figure 2: Mean squared error, normalized based on the maximum mean squared error which was encountered, for different numbers of neurons in the hidden layer of ParticleAreaNets. Each point represents the mean of ten measurements of the minimum mean squared error achieved on the test set during 200 epochs of training.

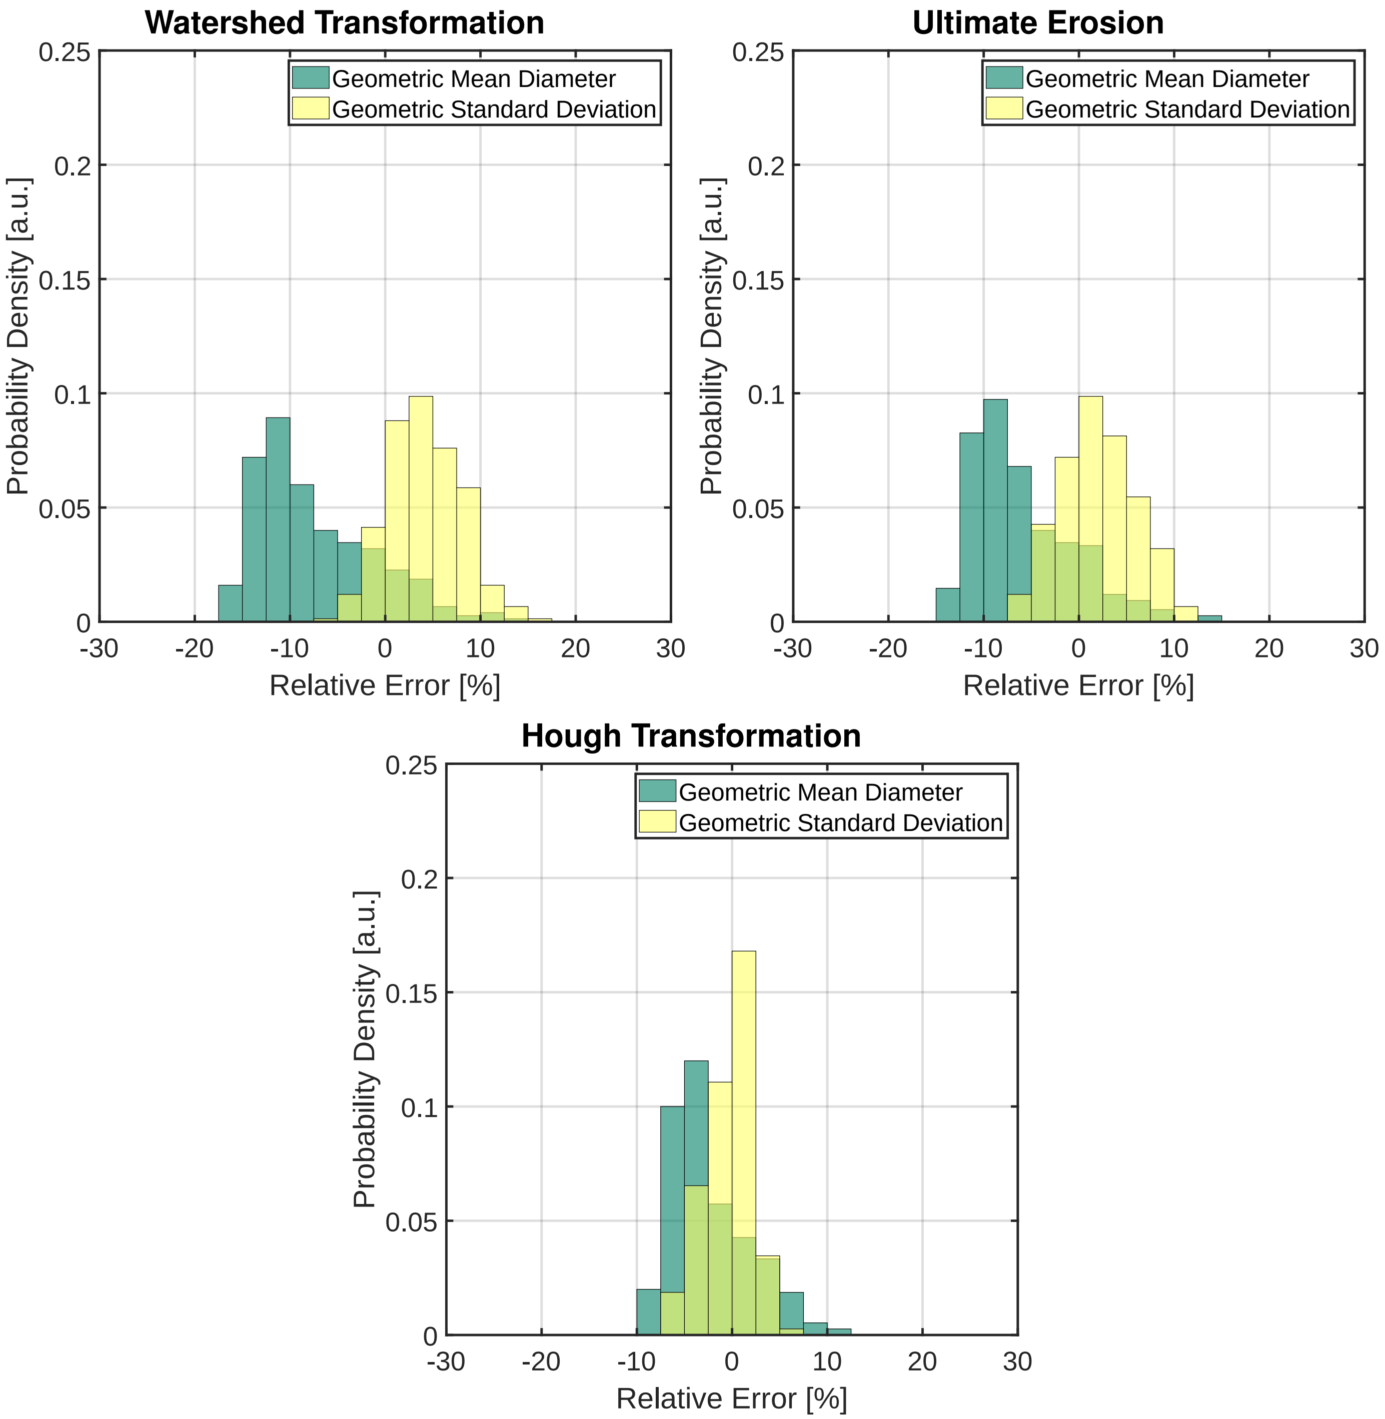


Figure 3: Histograms of the errors of the geometric mean diameter and the geometric standard deviation determined by three established automated methods when being applied to synthetic transmission electron microscopy images.

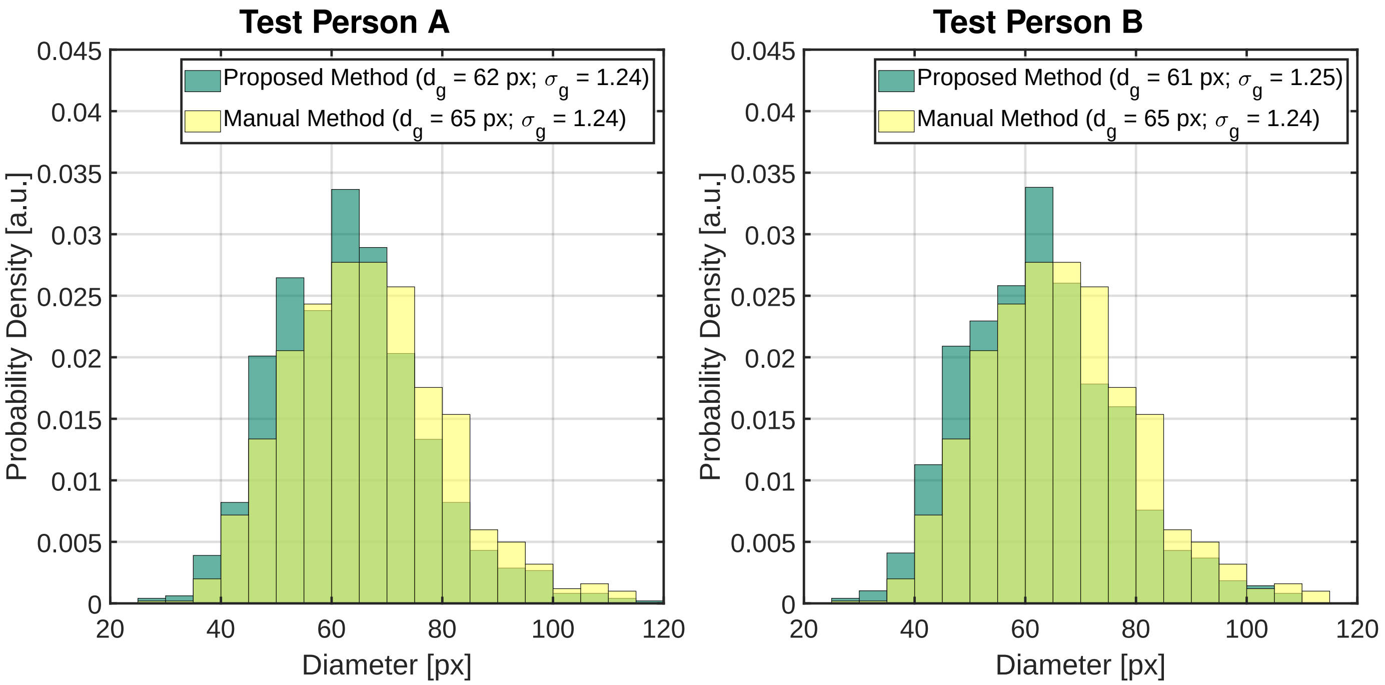


Figure 4: Particle size distributions acquired via the manual method being applied to synthetic transmission electron microscopy images by test person A (left) and test person B (right).
